# Supplementary material for: Blink: Lightweight Sample Runs for Cost Optimization of Big Data Applications
Source: arXiv:2207.02290 source file (2022-07-05)
Supplement: Supplementary file 3 [file appendix-c.tex]

% !TeX spellcheck = en_US
%-------------------------------------------------------------------------------
\section{Appendix C}
\label{sec:appendix-c}
%-------------------------------------------------------------------------------

%-------------------------------------------------------------------------------
% Commented part below.
%-------------------------------------------------------------------------------
